# Supplementary material for: Spin-orbit enabled all-electrical readout of chiral spin-textures
Source: arXiv:2202.11637 ancillary file (2022-02-23)
Supplement: Supplementary file 1 [file Supplement.pdf]

## **Supplementary Materials**

### **Spin-orbit enabled all-electrical readout of chiral spin-textures**

Imara Lima Fernandes, Stefan Blügel and Samir Lounis

## Supplementary Note 1 - Topological charge and helicity.

The topological charge  $\mathcal{Q}$  characterizes the topological nature of magnetic spin-textures by measuring the wrapping of the magnetization unit vector  $\mathbf{n}(\mathbf{r})$  around the unit sphere <sup>1</sup>:

$$\mathcal{Q} = \frac{1}{4\pi} \int \int d^2\mathbf{r} \quad \mathbf{n}(\mathbf{r}) \cdot \left[ \frac{\partial \mathbf{n}(\mathbf{r})}{\partial x} \times \frac{\partial \mathbf{n}(\mathbf{r})}{\partial y} \right]. \quad (1)$$

Besides the topological charge, the helicity  $\gamma$  and vorticity  $m$  are very instrumental to distinguish spin-textures sharing the same  $\mathcal{Q}$ . As reminder, here we give their definition following Ref. <sup>1</sup>. Utilizing spherical coordinates, the magnetization field of the magnetic texture can be expressed as:

$$\mathbf{n}(\mathbf{r}) = (\cos \Phi(\varphi) \sin \Theta(\mathbf{r}), \sin \Phi(\varphi) \sin \Theta(\mathbf{r}), \cos \Phi(\mathbf{r})) , \quad (2)$$

where the position vector  $\mathbf{r} = r(\cos \varphi, \sin \varphi)$  is given in polar coordinates. Then, by substituting  $\mathbf{n}(\mathbf{r})$  into Supplementary Equation 1, we obtain:

$$\mathcal{Q} = - \left[ \frac{\cos \Theta(r)}{2} \right]_{r=0}^{r=\infty} \left[ \frac{\Phi(\varphi)}{2\pi} \right]_{\varphi=0}^{\varphi=2\pi}. \quad (3)$$

In general, the magnetic moment at the skyrmion's core points down, i.e.,  $\Theta(0) = \pi$ , while the moments at the periphery of the magnetic structure point up, i.e.,  $\Theta(r \rightarrow \infty) = 0$ . Thus,  $\left[ \cos \Theta(r)/2 \right]_{r=0}^{r=\infty} = 1$ . Meanwhile, the vorticity is defined as  $m = [\Phi(\varphi)/2\pi]_{\varphi=0}^{\varphi=2\pi}$ . Considering the boundary conditions at  $r \rightarrow \infty$  fixed, the vorticity determines the topological charge as  $\mathcal{Q} = -m$ . In addition, the helicity can be defined as phase  $\gamma$  in

$$\Phi(\varphi) = m\varphi + \gamma. \quad (4)$$

## Supplementary Note 2 - Multiple-scattering expansion of the LDOS.

We invoke multiple-scattering theory to demonstrate that upon rotation of magnetic moments at the neighborhood of a given atomic moment  $i$ , the local density of states (LDOS) will experience modifications intimately related to the electron scattering among the canted spin moments. Starting without loss of generality with the hamiltonian  $H$  of a non-magnetic system without spin-orbit coupling (SOC), the Green function is simply defined as  $G(E) = (E - H)^{-1}$ , from which the LDOS at a given site  $i$  can be extracted:

$$\text{LDOS}_i(E) = -\frac{1}{\pi} \text{Im Tr } G_{ii}(E), \quad (5)$$

where the trace is taken over the orbital and spin angular momenta indices.

If the atoms carry magnetic moments, the atomic potentials are modified by an additional  $v_i = U_i(\mathbf{S}_i \cdot \boldsymbol{\sigma})$  for each site  $i$ , where  $U$  defines the atomic exchange splitting, while SOC gives rise to  $v_i^{\text{so}} = \lambda_i(\mathbf{L}_i \cdot \boldsymbol{\sigma})$ .  $\mathbf{S}$  is the unit vector of the magnetic moment,  $\lambda$  represents the strength of SOC on site  $i$  between the electron spin and its atomic orbital angular momentum  $\mathbf{L}_i$  while  $\boldsymbol{\sigma}$  is the vector of Pauli matrices. The impact of magnetism and SOC on the electronic structure can be tracked via the Dyson equation, which relates the new Green function  $g$  to the original one  $G$ :

$$g = G + Gvg = G + GvG + GvGvG + GvGvGvG + \dots, \quad (6)$$

where we performed Born iterations.

The expansion to second order  $GvGvG$  gives rise to the two-site isotropic spin-mixing magnetoresistance (I-XMR), which does not require SOC as discussed in the main text. Using known

relations involving products of Pauli matrices:  $(\mathbf{a} \cdot \boldsymbol{\sigma})(\mathbf{b} \cdot \boldsymbol{\sigma}) = (\mathbf{a} \cdot \mathbf{b}) \sigma_0 + i(\mathbf{a} \times \mathbf{b}) \cdot \boldsymbol{\sigma}$ , we find that one of the terms contributing to the LDOS looks like

$$-\frac{1}{\pi} \text{Im Tr } G_{ij}(E) U_j(\mathbf{S}_j \cdot \boldsymbol{\sigma}) G_{ji}(E) U_i(\mathbf{S}_i \cdot \boldsymbol{\sigma}) G_{ii}(E), \quad (7)$$

yielding the general expansion

$$\text{LDOS}_i^{(2) \text{ I-XMR}}(E) = \sum_j f_{ij}^{(2) \text{ I-XMR}}(E) (\mathbf{S}_i \cdot \mathbf{S}_j). \quad (8)$$

for the two-site two-spin scattering term with  $f_{ij}^{(2) \text{ I-XMR}}(E) = -\frac{2}{\pi} \text{Im Tr } G_{ij}(E) U_j G_{ji}(E) U_i G_{ii}(E)$ .

We also uncover isotropic SOC-independent higher-order scattering terms such as the 4-spin contribution:

$$\text{LDOS}_i^{(4) \text{ I-XMR}}(E) \propto \sum_{jkl} f_{ijkl}^{(4) \text{ I-XMR}}(E) [(\mathbf{S}_i \cdot \mathbf{S}_j)(\mathbf{S}_k \cdot \mathbf{S}_l) - (\mathbf{S}_i \cdot \mathbf{S}_k)(\mathbf{S}_j \cdot \mathbf{S}_l) + (\mathbf{S}_i \cdot \mathbf{S}_l)(\mathbf{S}_j \cdot \mathbf{S}_k)], \quad (9)$$

which simplified to a biquadratic contribution if one limits the expansion to a two-site scattering event, as considered in the main text.

The third order term in the expansion of the Dyson equation gives rise to a chiral contribution when the scattering involves two magnetic sites and a third site carrying SOC. For instance, one of the terms looks like

$$\begin{aligned} & -\frac{1}{\pi} \text{Im Tr } G_{ij}(E) v_j G_{jk}(E) v_k^{\text{so}} G_{ki}(E) v_i G_{ii}(E) \\ &= -\frac{1}{\pi} \text{Im Tr } G_{ij}(E) U_j(\mathbf{S}_j \cdot \boldsymbol{\sigma}) G_{jk}(E) \lambda_k (\mathbf{L}_k \cdot \boldsymbol{\sigma}) G_{ki}(E) U_i(\mathbf{S}_i \cdot \boldsymbol{\sigma}) G_{ii}(E) \\ &= -\frac{2}{\pi} \text{Re Tr } G_{ki}(E) U_i G_{ii}(E) G_{ij}(E) U_j G_{jk}(E) \lambda_k \mathbf{L}_k \cdot (\mathbf{S}_i \times \mathbf{S}_j). \end{aligned} \quad (10)$$

Thus in general, we expect a chiral dependence of the LDOS:

$$\text{LDOS}_i^{\text{C-XMR}}(E) = \sum_j \mathbf{f}_{ij}^{\text{C-XMR}}(E) \cdot (\mathbf{S}_i \times \mathbf{S}_j), \quad (11)$$

which is linear with SOC similarly to the Dzyaloshinskii-Moriya interaction (DMI)<sup>2,3</sup>.  $\mathbf{f}_{ij}^{\text{C-XMR}}(E)$  is the analog of the DMI vector and thus its direction obeys the same symmetry rules and its existence requires broken inversion symmetry.

Interestingly, a fourth-order scattering term (second-order scattering at magnetic and SOC sites), quadratic with respect to SOC, leads to the usual anisotropic magnetoresistance contribution, if the scattering occurs on the same site (local contribution). A non-local contribution is however possible, which gives rise to the anisotropic XMR (X-AMR). The conventional AMR can be expressed as:

$$\text{LDOS}_i^{\text{AMR}}(E) = (\mathbf{S}_i \cdot \mathbf{f}_i^{\text{X-AMR}}(E))^2, \quad (12)$$

where  $\mathbf{f}^{\text{X-AMR}}$  represents the anisotropy field. This leads to the usual phenomenological form  $\cos^2 \theta_i$  characterizing the AMR signal, where theta is the polar angle of the magnetic moment at site  $i$  with respect to  $\mathbf{f}$ .

Besides the local contribution, there are various possible non-local terms shaping the total AMR. Their form emerging from a two-site scattering event can be written as:

$$\text{LDOS}_i^{\text{X-AMR}}(E) = \sum_{j \neq i} (\mathbf{S}_i \cdot \mathbf{f}_j^{\text{X-AMR}}(E)) (\mathbf{S}_j \cdot \mathbf{f}_i^{\text{X-AMR}}(E)). \quad (13)$$

As it can be recognized, the angular dependence of the X-AMR is different from the AMR one:  $\cos \theta_i \cos \theta_j$  instead of  $\cos^2 \theta_i$ .

Finally, we get a correction to the I-XMR contribution, which is quadratic with SOC, dubbed here anisotropic XMR (Ani-XMR):

$$\text{LDOS}_i^{\text{Ani-XMR}}(E) \propto \sum_{j \neq i} f_{ij}^{\text{Ani-XMR}}(E) (\mathbf{S}_i \cdot \mathbf{S}_j), \quad (14)$$

where  $f^{\text{AniXMR}}$  is a scalar quantity that depends on SOC.

### Supplementary Note 3 - XMR efficiency without SOC – I-XMR.

The XMR efficiency is obtained by taking the difference of the LDOS decaying into vacuum (probed by the STM tip) between the two cases: non-collinear (NC) versus collinear (C) spin states. The difference is then normalized by the collinear LDOS:

$$\text{XMR}^\gamma(E) = \frac{\text{LDOS}_{\text{NC}}^\gamma(E) - \text{LDOS}_{\text{C}}(E)}{\text{LDOS}_{\text{C}}(E)} \quad (15)$$

where  $\gamma$  indicates the helicity of the skyrmion.

Following Supplementary Equation 8 and 9, the XMR effect without SOC contribution at a position  $i$  is found to depend on the dot-product with the surrounding 6 nearest neighbor spins,

$$\text{I-XMR}(E) \approx \gamma_{\text{I-XMR}}^{2\text{-spin}}(E) \sum_{j \in \text{NN}} \mathbf{S}_i \cdot \mathbf{S}_j + \gamma_{\text{I-XMR}}^{4\text{-spin}}(E) \sum_{j \in \text{NN}} (\mathbf{S}_i \cdot \mathbf{S}_j)^2 - 6 \left( \gamma_{\text{I-XMR}}^{2\text{-spin}}(E) + \gamma_{\text{I-XMR}}^{4\text{-spin}}(E) \right), \quad (16)$$

where  $\gamma_{\text{I-XMR}}$  describes the I-XMR weight that one can extract from a fit of the measured transport spectra.

We collect the sum of the dot products of each of the magnetic moments with their respec-

tive 6 nearest neighbors and plot the corresponding atomically resolved I-XMR in Supplementary Figure 1 at different bias voltages. The red circles represent the values obtained from our *ab initio* calculations for each atom within the Néel-type skyrmion with diameter  $D_{Sk} \approx 2.2$  nm. The straight lines represent a good fit to the *ab initio* data, which provide a reasonable estimate of  $\gamma_{\text{I-XMR}}$ .

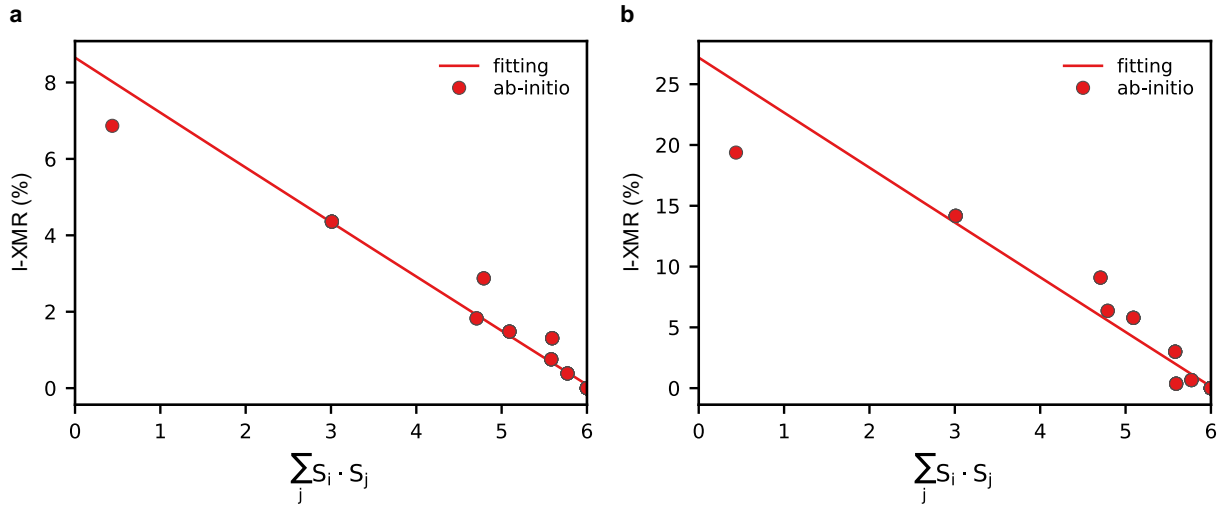

**Supplementary Figure 1: Fit of the I-XMR weight.** First-principles results (circles) of the I-XMR effect at a particular tunneling energy **a**  $eV_{\text{bias}} = 0.21$  eV and **b**  $eV_{\text{bias}} = 0.52$  eV as function of the sum of the dot product of nearest neighboring spin moments. These results are then fitted following Supplementary Equation 16 (solid line).

#### Supplementary Note 4 - Chiral spin-mixing magnetoresistance – C-XMR.

Following Supplementary Equation 11, the C-XMR efficiency can be written as

$$\text{C-XMR}_i(E) \approx \gamma_{\text{C-XMR}}(E) \sum_{j \in \text{NN}} \hat{\mathbf{c}}_{ij} \cdot \mathbf{S}_i \times \mathbf{S}_j, \quad (17)$$

assuming the contribution of nearest neighbors to site  $i$  and where  $\hat{c}$  is a chirality vector parallel to  $\mathbf{f}^{\text{C-XMR}}$ .  $\hat{c}$  obeys the same symmetry rules dictating the direction of the DMI. In the particular case studied in the paper, the in-plane components of  $\hat{c}$  follow those of the DM vector. The  $z$ -component is however unknown. Thus, we choose here to modulate that component by a factor of  $\alpha$  with respect to that of the DM vector (see Supplementary Figure 2a-c).

In order to quantify  $\gamma_{\text{C-XMR}}$ , we proceed to a fit similarly to what was done in the previous Note. Here, however, the ab-initio obtained data will be shifted laterally depending on  $\alpha$  as plotted in Supplementary Figure 2d-e. Since the  $z$ -component of the DMI vector is rather small, there are no significant differences among the data points associated with the three values considered for  $\alpha$ : 1.0 (red dots), 0.5 (blue dots) and 0.0, i.e. with purely in-plane  $\hat{c}$  (green circles). Once more the linear fit seems reasonable. If there is mismatch, it can be assigned to the chiral scattering contribution from second nearest neighbors of higher-order chiral contributions.

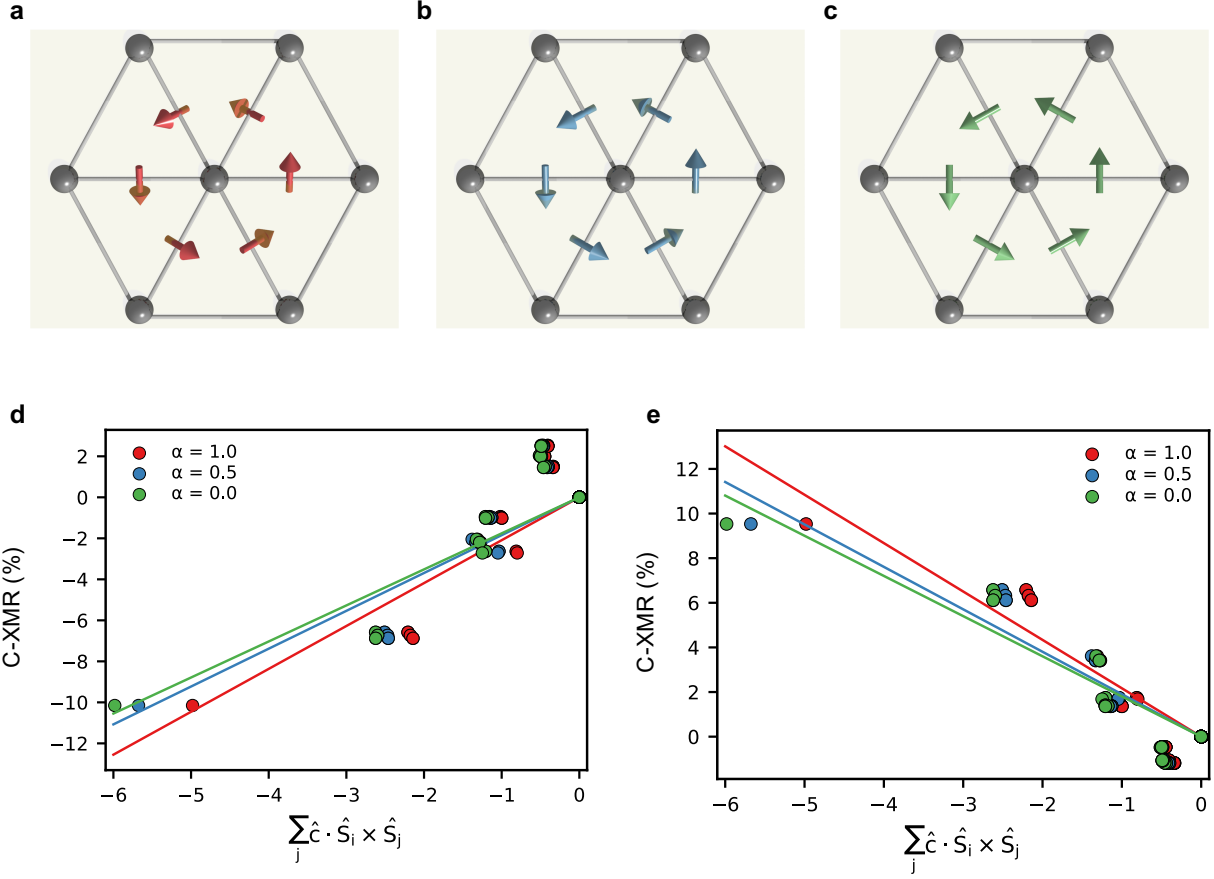

**Supplementary Figure 2: Fit of the C-XMR weight.** The  $\hat{c}$  vector follows the orientation of the DMI-vector with the z-component scaled by the factor **a**  $\alpha = 1.0$  (red), **b**  $\alpha = 0.5$  (blue) and **c**  $\alpha = 0.0$  (green). First-principles results (circles) of the C-XMR effect at a particular tunneling energy **d**  $eV_{\text{bias}} = 0.61$  eV and **e**  $eV_{\text{bias}} = 0.89$  eV as function of the cross product of  $\mathbf{S}_i$  with the surrounding 6 nearest neighbor spins. These results are then fitted (solid lines) according to Supplementary Equation 17, considering the factor  $\alpha = 1.0$  (red),  $\alpha = 0.5$  (blue) and  $\alpha = 0.0$  (green).

## Supplementary Note 5 - Anisotropic magnetoresistances – AMR, X-AMR and Ani-XMR.

Starting with Supplementary Equation 13-14 and limiting the scattering contributions to the nearest neighbors, the total AMR, which is biquadratic with SOC, at a site  $i$  contains three contributions:

$$\begin{aligned} \text{AMR}_{\text{total}}^i(E) &\approx \gamma_{\text{AMR}}(E) \cos^2 \theta_i + \gamma_{\text{X-AMR}}(E) \sum_{j \in \text{NN}} \cos \theta_i \cos \theta_j + \gamma_{\text{Ani-XMR}}(E) \sum_{j \in \text{NN}} \mathbf{S}_i \cdot \mathbf{S}_j \\ &- (\gamma_{\text{AMR}}(E) + 6\gamma_{\text{X-AMR}}(E) + 6\gamma_{\text{Ani-XMR}}(E)) , \end{aligned} \quad (18)$$

where  $\theta_i$  is the polar angle associated with the magnetic moment at site  $i$ .

In general the non-local contribution, X-AMR, provides the largest weight to the total AMR. An example of a fitting procedure to extract the various weights is illustrated in Supplementary Figure 3. We proceed to the different fits in a sequential fashion. We start by extracting  $\gamma_{\text{X-AMR}}$  (Supplementary Figure 3a,d). The rest of the signal  $\text{AMR}_{\text{total}} - \text{X-AMR}$  is then fitted to obtain  $\gamma_{\text{AMR}}$  (Supplementary Figure 3b,e). Finally, we conclude with the last weight  $\gamma_{\text{Ani-XMR}}$  (Supplementary Figure 3c,f).

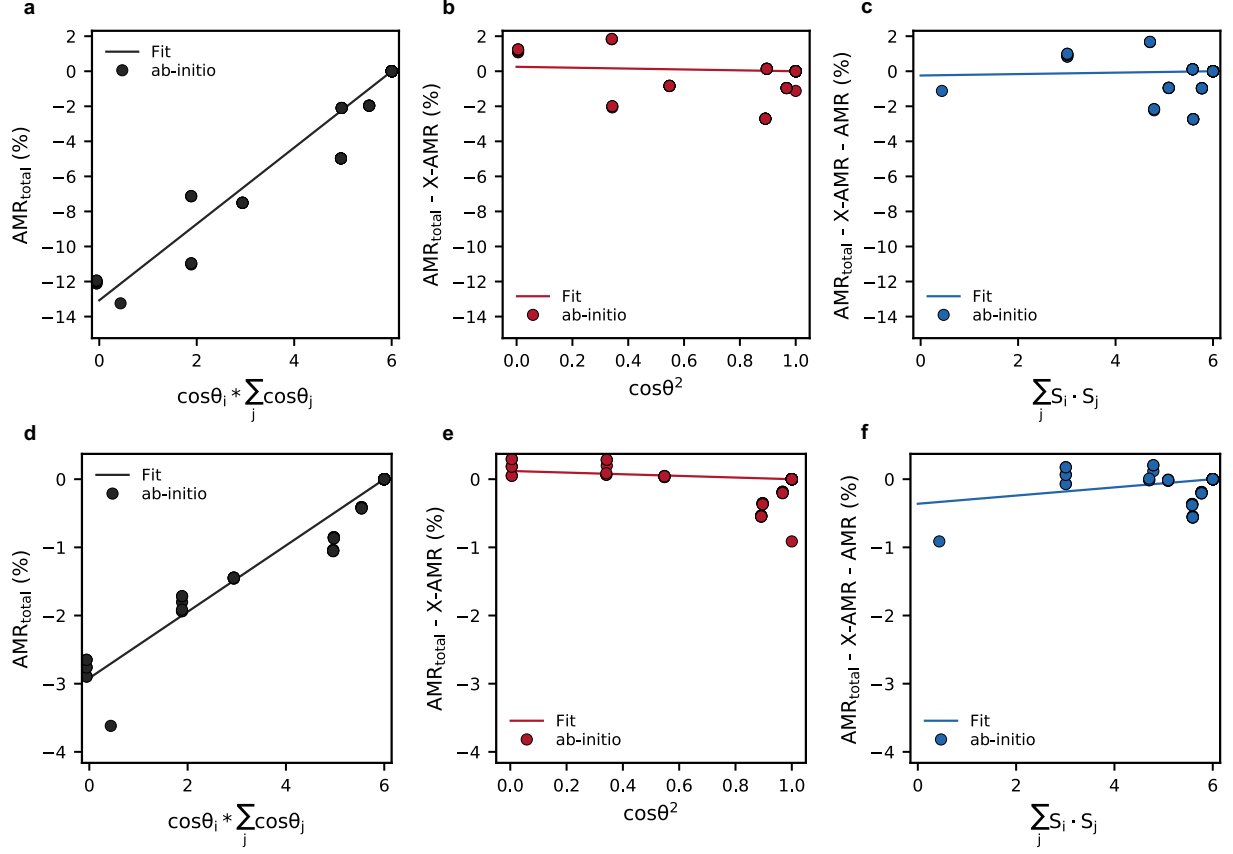

**Supplementary Figure 3: Fit of the family of AMR weights.** First-principles results (black circles) of the total AMR at site  $i$  at a tunneling energy **a**  $eV_{bias} = -1.29$  eV (**d**  $eV_{bias} = 1.01$  eV) as function of the sum of products  $\cos\theta_i \cos\theta_j$  with the surrounding 6 nearest neighbor spins. These results are then fitted to extract  $\gamma_{X-AMR}$  (solid black line). The remaining local (conventional) AMR and anisotropic XMR weights are obtained in **b** (**e**) and **c** (**f**) respectively.

## Supplementary Note 6 - Magnetoresistances associated with various skyrmionic structures.

The various MR patterns hosted by Neel with helicity  $\gamma = \pi$ , Bloch skyrmions and antiskyrmions at 0.61 eV are illustrated in Supplementary Figures 4-6, respectively. One can clearly see that the C-XMR effect can be used to distinguish skyrmionic structures while all other MRs are identical since they are independent of the chirality/helicity of the spin-textures.

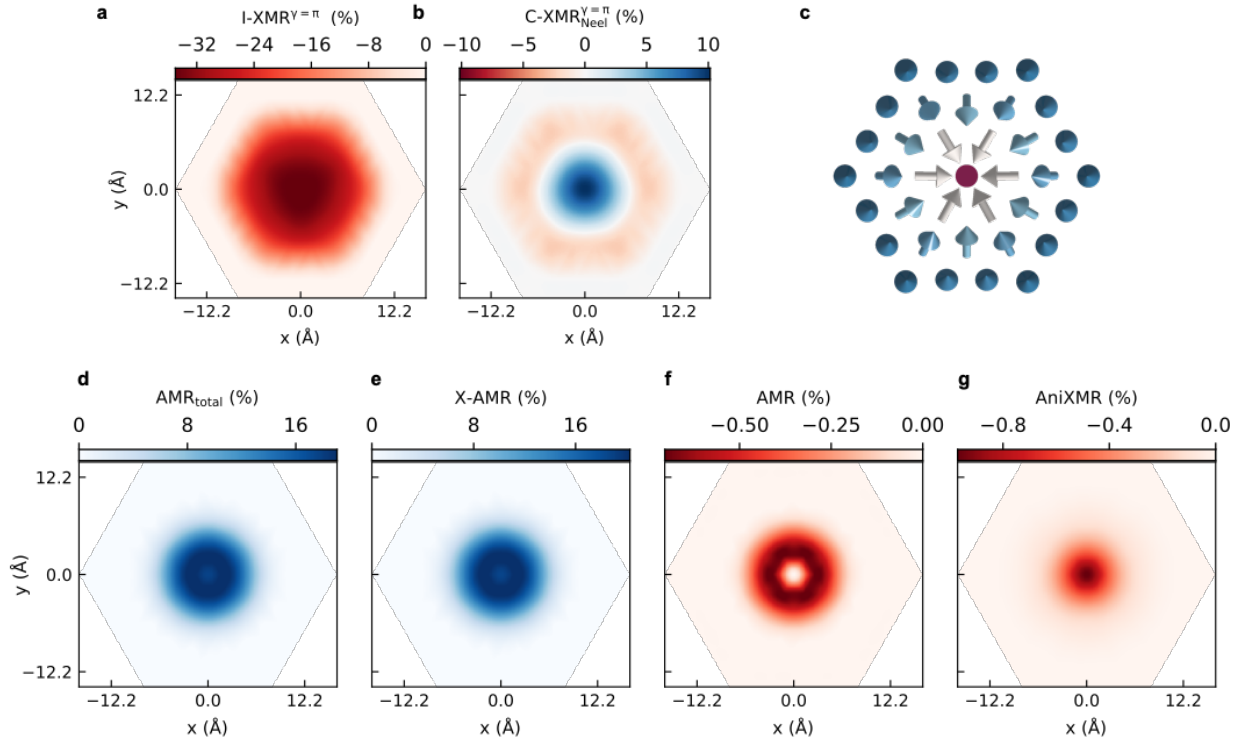

**Supplementary Figure 4: Magnetoresistance patterns characterizing a Néel skyrmion with  $\gamma = \pi$ .** **a-b** Spin-orbit independent XMR pattern compared to the one emerging from C-XMR as obtained at the energy bias of  $eV_{\text{bias}} = 0.61$  eV. **c** Néel-type skyrmion with helicity  $\gamma = \pi$ . **d** Total AMR signal decomposed into the **e** X-AMR, **f** conventional AMR, and **g** ani-XMR components.

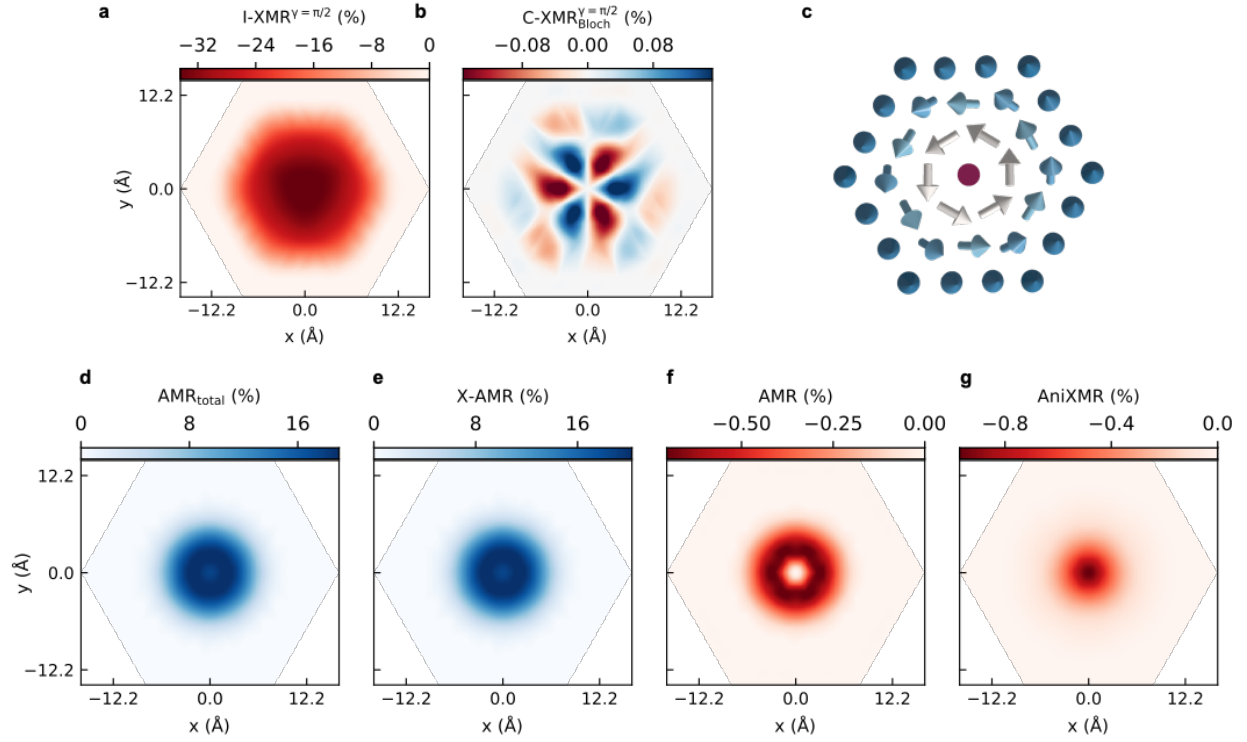

**Supplementary Figure 5: Magnetoresistance patterns characterizing a Bloch skyrmion.** **a-b** Spin-orbit independent XMR pattern compared to the one emerging from C-XMR as obtained at the energy bias of  $eV_{\text{bias}} = 0.61$  eV. **c** Bloch-type skyrmion with helicity  $\gamma = \pi/2$ . **d** Total AMR signal decomposed into the **e** X-AMR, **f** conventional AMR, and **g** ani-XMR components.

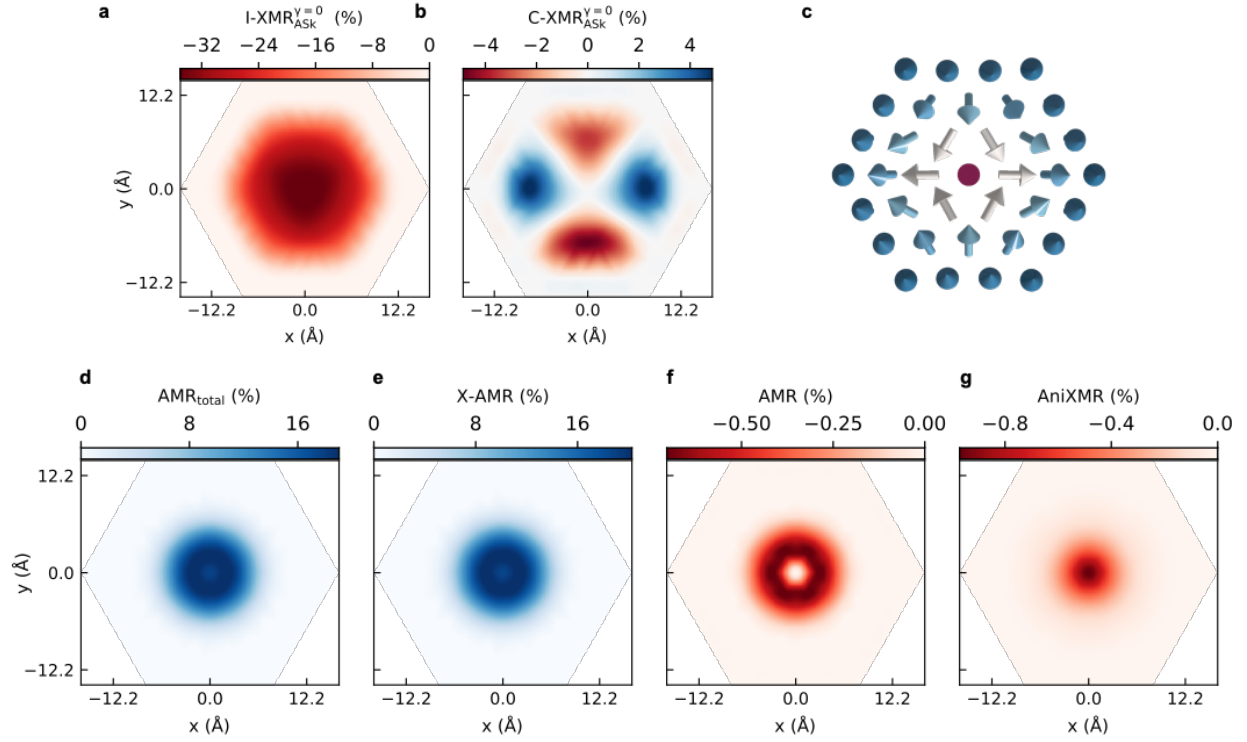

**Supplementary Figure 6: Magnetoresistance patterns characterizing an Anti-skyrmion. a-b** Spin-orbit independent XMR pattern compared to the one emerging from C-XMR as obtained at the energy bias of  $eV_{\text{bias}} = 0.61$  eV. **c** Anti-skyrmion with helicity  $\gamma = 0$ . **d** Total AMR signal decomposed into the **e** X-AMR, **f** conventional AMR, and **g** ani-XMR components.

## Supplementary References

1. Nagaosa, N. & Tokura, Y. Topological properties and dynamics of magnetic skyrmions. *Nat. Nanotech.* **8**, 899–911 (2013).
2. Dzyaloshinsky, I. A thermodynamic theory of “weak” ferromagnetism of antiferromagnetics. *J. Phys. Chem. Sol.* **4**, 241 – 255 (1958).
3. Moriya, T. Anisotropic superexchange interaction and weak ferromagnetism. *Phys. Rev.* **120**, 91–98 (1960).
